# Supplementary material for: Give Me More Details: Improving Fact-Checking with Latent Retrieval
Source: arXiv:2305.16128 source file (2024-01-27)
Supplement: Supplementary file 1 [file 9_appendix.tex]

\section{Graph-based Model}\label{Graph-based Model}
In this section, we describe the Kernel Graph Attention Network (KGAT) \cite{Liu2020KernelGA} and how to use it for claim verification. KGAT creates an evidence graph for claim $c$ by extracting evidence sentences $D=\{e^{1},...,e^{p},...,e^{l}\}$, and then utilizes the evidence graph to predict the claim label $y$.

KGAT builds the evidence graph $G$ by making each claim-evidence pair a node and connecting all node pairs with edges, resulting in a fully connected evidence graph with $l$ nodes as: $N=\{n^{1},...,n^{p},...,n^{l}\}$.

KGAT combines multiple and single evidence reasoning scenarios to generate a probability $P(y|c,D)$ for predicting the claim label $y$. In a graph neural network, KGAT uses the graph attention operation~\cite{Velickovic2018GraphAN} and splits the prediction into two parts: (1) the label prediction in each node conditioned on the whole graph $P(y|n^{p},G)$; (2) the evidence selection probability $P(n^{p}|G)$:
\begin{equation}
   P(y \mid c, D)=\sum_{p=1}^{l} P\left(y \mid c, e^{p}, D\right) P\left(e^{p} \mid c, D\right) 
\end{equation}
or in the graph notation:
\begin{equation}
P(y \mid G)=\sum_{p=1}^{l} P\left(y \mid n^{p}, G\right) P\left(n^{p} \mid G\right).
\end{equation}

The joint reasoning probability $P(y|n^{p},G)$ calculates node label prediction with multiple evidence. The readout module \cite{knyazev2019understanding} calculates the probability $P(n^{p}|G)$ and attentively combines per-node signals for prediction.

% Moreover, we can also apply the method of kernel graph attention network to low-resource relation extraction \cite{hu2020selfore,GuoN0C20, hu2021gradient,hu2021semi,liu2022hierarchical}, natural language inference \cite{li2023multi,li2022pair}, semantic parsing \cite{liu2022semantic,liu2023comprehensive}, and other NLP application tasks, thus realizing reasoning enhancement based on graph structure.

\section{Pipeline and Joint Extractors Baselines}\label{pipeline_baseline}

\subsubsection{Pipeline Extractors}

\noindent \textbf{(1) Rule-based Extractor}: This is a simple baseline that only includes the $N$ sentences surrounding the snippet in the source document. In practice, we choose $N=6$ and $N=12$. 

\noindent \textbf{(2) Surface Extractor}: Following previous efforts on synthetic datasets~\citep{Thorne2018FEVERAL,jiang2020hover,Aly2021FEVEROUSFE}, we use TF-IDF to extract sentences in the documents as the evidence.

\noindent \textbf{(3) Semantic Extractor}:  
Following~\citet{Nie2019CombiningFE}, we extract evidence based on semantic similarity. BERT~\citep{Devlin2019BERTPO} is used to get the representations of the claim and sentences in the document. Cosine similarity is used for selection.

\noindent \textbf{(4) Hybrid Extractor}: 
Prior work show that semantic similarity can be complementary to surface form matching~\citep{Shaar2020ThatIA}. Therefore, we use rankSVM to select sentences based on the feature sets of rankings returned by TF-IDF and the similarity scores computed with BERT.

\noindent \textbf{(5) CONCRETE}: \citet{huang2022concrete} introduces a pioneering fact-checking framework utilizing cross-lingual retrieval, gathering evidence from various languages using a retriever.

\noindent \textbf{(6) CofCED}: \citet{yang2022coarse} employs a hierarchical encoder for web text representation, develops cascaded selectors for verdict-explainable sentence selection.

\subsubsection{Joint Extractors}

\noindent \textbf {(1) Attention}: Following~\citet{gupta-srikumar-2021-x}, we calculate relevance weights between the output embeddings of all retrieved sentences and the claim via dot product attention. Then we obtain the evidence by filtering the weighted sentences.

\noindent \textbf{(2) Reinforce}: We follow~\citet{LeiBJ16} by assigning a binary Bernoulli variable to each sentence from source documents. The evidence extractor is optimized using REINFORCE~\citep{williams1992simple}. A $L_{0}$ regularizer is used to impose sparsity.

\noindent \textbf{(3) FusedMax}: We used fusedmax~\citep{NiculaeB17} to encourage attention to contiguous segments of text, by adding an additional total variation regularizer, inspired by the fused lasso.

\noindent \textbf{(4) Gumbel}: Following~\citet{maddisonMT17}, we employ the Gumbel-Max trick to reparameterize the Bernoulli variables.

\noindent \textbf{(5) HardKuma}: We follow~\citet{BastingsAT19} by adopting HardKuma variables and use reparameterized gradients estimates for jointly training~\citep{KingmaW14}.

\noindent \textbf{(6) UNIREX}: We adopt the rationale extraction method in \citet{chan2022unirex}.
